# Supplementary material for: Limited Resources Induce Bistability in Microtubule Length Regulation
Source: arXiv:1802.09265 source file (2018-04-09)
Supplement: Supplementary file 1 [file supplement_final.pdf]

# Supplemental Materials: Limited Resources Induce Bistability in Microtubule Length Regulation

Matthias Rank,[1,*] Aniruddha Mitra,[2,3,*] Louis Reese,[4] Stefan Diez,[2,3,†] and Erwin Frey[1,‡]

[1]*Arnold-Sommerfeld-Center for Theoretical Physics and Center for NanoScience, Ludwig-Maximilians-Universität München, Theresienstraße 37, 80333 München, Germany*

[2]*B CUBE – Center for Molecular Bioengineering and Center for Advancing Electronics Dresden (cfaed), Technische Universität Dresden, Arnoldstraße 18, 01307 Dresden, Germany*

[3]*Max Planck Institute of Molecular Cell Biology and Genetics, Pfotenhauerstraße 108, 01307 Dresden, Germany*

[4]*Department of Bionanoscience, Kavli Institute of Nanoscience, Faculty of Applied Sciences, Delft University of Technology, Van der Maasweg 9, 2629 HZ Delft, The Netherlands*

## CONTENTS

S.I. Brief review of TASEP/LK 1

S.II. Full mean-field solution based on TASEP/LK 2
- A. Reduction to a lattice of constant length 2
- B. Strategy to obtain the stationary state 3
- C. Case $K > 1$ 3
  - 1. Low density/high density (LD/HD) phase 3
  - 2. Low density (LD) phase 4
- D. Case $K < 1$ 6
  - 1. Low hole density/high hole density (LhD/HhD) phase 6
  - 2. High hole density (HhD) phase 6
- E. Comparison with simulations, and the phase diagram/stability diagram 7

S.III. Estimation of the parameters 8

S.IV. Robustness of the parameters $\delta$ and $V$ 8

S.V. Many MTs with shared reservoirs 10
- A. Shared reservoirs with infinitely fast diffusion 10
- B. Shared reservoirs with finite diffusion 12

S.VI. Experimental Methods 15

S.VII. Variability in experimental data 15

S.VIII. Supplementary Figures 17

References 20

* These authors contributed equally
† stefan.diez@tu-dresden.de
‡ frey@lmu.de

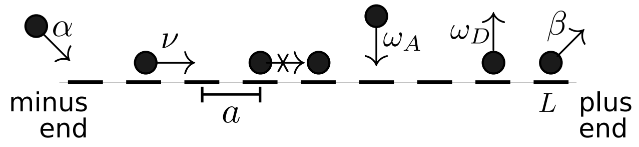


FIG. S1. The totally asymmetric simple exclusion process with Langmuir kinetics (TASEP/LK). Particles jump to the right at rate $\nu$, provided the next site is empty. They attach to the lattice at $\omega_\mathrm{A}$; in addition, particles may enter at the left end of the lattice end at $\alpha$ if the first site is unoccupied. Particles leave the lattice by exiting at the right end at rate $\beta$, or by detaching from any other site at $\omega_\mathrm{D}$.

## S.I. BRIEF REVIEW OF TASEP/LK

The totally asymmetric simple exclusion process with Langmuir kinetics (TASEP/LK), on which our model presented in the main text is based, is schematically depicted in Fig. S1. In the lattice bulk, the stochastic processes in TASEP/LK are identical to those of our model, cf. Fig. 1b in the main text. In TASEP/LK, using the notation of Refs. [1, 2], the attachment rate $\omega_\mathrm{A}$ is constant, i.e. one assumes that the motor reservoir is unlimited. The detachment rate in the lattice bulk is given by $\omega_\mathrm{D}$. Particles move to the next site a distance $a$ apart at rate $\nu$. At the left end, which corresponds to the minus end of the MT, Fig. 1b in the main text, particles enter the lattice at rate $\alpha$ if the first site is not occupied; at the right end (the plus end), particles leave the lattice at rate $\beta$. Note that unlike for the stochastic model in the main text, in TASEP/LK, particle detachment at the plus end preserves the lattice integrity, i.e., its length $L$ remains constant.

For TASEP/LK, the density profile of particles on the lattice is well known. Depending on the parameters $K = \omega_\mathrm{A}/\omega_\mathrm{D}$, $\Omega_\mathrm{D} = \omega_\mathrm{D} L$, and the rates $\alpha$ and $\beta$, the profile can look very different. While we refer the reader to Ref. [2] for full details of the mathematical analysis, here we summarize the main aspects of TASEP/LK model which are of relevance for our study.

Identical to the main text, Eq. (3), the motor density

in the lattice bulk in the stationary state follows from

$$\partial_t\rho_i = \nu\left[\rho_{i-a}(1-\rho_i) - \rho_i(1-\rho_{i+a})\right] + \omega_\mathrm{A}(1-\rho_i) - \omega_\mathrm{D}\rho_i = 0 \ , \tag{S1}$$

where we have employed the mean field approximation $\langle n_i n_j\rangle \approx \langle n_i\rangle\langle n_j\rangle = \rho_i\rho_j$, and $\rho_i$ is the average motor density at the site located at $i \in \{0, a, 2a, \dots, L\}$. The boundary conditions are given by

$$0 = \partial_t\rho_0 = \alpha(1-\rho_0) - \nu\rho_0(1-\rho_a), \tag{S2a}$$

at the minus end of the lattice, and

$$0 = \partial_t\rho_L = \nu\rho_{L-a}(1-\rho_L) - \rho_L\beta \tag{S2b}$$

at the plus end. Like in the main text, we perform the continuum limit for Eqs. (S1) and (S2) [2], and obtain [3]

$$a\nu\left[\partial_x\sigma(x) + \partial_x \ln|\sigma(x)|\right] = \omega_\mathrm{D}\frac{(K+1)^2}{K-1}, \tag{S3}$$

where the density $\rho$ and the "reduced density" $\sigma$ are related as

$$\sigma = \frac{K+1}{K-1}(2\rho-1) - 1 \ . \tag{S4}$$

In the continuous description, the boundary conditions following from Eq. (S2) are $\rho(0) = \alpha/\nu$, and $\rho(L) = 1 - \beta/\nu$.

Provided $K = \omega_\mathrm{A}/\omega_\mathrm{D} > 1$, the solutions of Eq. (S3) can be obtained in terms of the different branches of the Lambert $W$ function [2], which is defined as the inverse function of $f(x) = xe^x$. For the opposite case, $K < 1$, a solution can be obtained by exploiting the particle-hole symmetry of the TASEP/LK model: The model maps onto itself by changing the spatial coordinate $x \leftrightarrow L - x$ and the density $\rho \leftrightarrow 1 - \rho$, and simultaneously interchanging $\alpha$ and $\beta$, and $\omega_\mathrm{A}$ and $\omega_\mathrm{D}$ [2].

In terms of the two branches of the Lambert $W$ function, $W_0$ and $W_{-1}$, the reduced density profile in case $K > 1$ can be written as [2]

$$\sigma_\alpha(x) = W_{-1}(-Y_\alpha(x)) \tag{S5a}$$

and

$$\sigma_\beta = \begin{cases} W_0(Y_\beta(x)) \ , & \text{if } 0 \le \frac{\beta}{\nu} < 1 - \frac{\omega_\mathrm{A}}{\omega_\mathrm{A}+\omega_\mathrm{D}} \\ 0 \ , & \text{if } \frac{\beta}{\nu} = 1 - \frac{\omega_\mathrm{A}}{\omega_\mathrm{A}+\omega_\mathrm{D}} \\ W_0(-Y_\beta(x)) \ , & \text{if } 1 - \frac{\omega_\mathrm{A}}{\omega_\mathrm{A}+\omega_\mathrm{D}} < \frac{\beta}{\nu} < \frac{1}{2} \end{cases} \tag{S5b}$$

with the function $Y(x)$ defined as

$$Y(x) = |\sigma(x_0)| \exp\left[\frac{\omega_\mathrm{D}}{\nu}\frac{(K+1)^2}{K-1}\frac{(x-x_0)}{a} + \sigma(x_0)\right] \ , \tag{S6}$$

and $Y_\alpha$ and $Y_\beta$ are the solutions in which the reduced density $\sigma(x_0)$ is evaluated at $x_0 = 0$, or $x_0 = L$, respectively.

In Ref. [2] it was shown that among others [4] there are three possible solutions for the actual density profile:

(i) The density profile $\rho(x)$ is given by $\rho_\alpha(x)$ along the whole lattice, and has a discontinuity at the plus end; this is called the low density (LD) phase, see Fig. S4a.

(ii) The density profile $\rho(x)$ is given by $\rho_\beta(x)$ along the whole lattice, and has a discontinuity at the minus end; this is called the high density (HD) phase.

(iii) The density profile $\rho(x)$ is given by $\rho_\alpha(x)$ in the vicinity of the minus end, and $\rho_\beta(x)$ near the plus end. At position $x_w$, the density $\rho(x)$ increases discontinuously from $\rho_\alpha(x_w)$ to $\rho_\beta(x_w)$, and $\rho_\alpha(x_w) = 1 - \rho_\beta(x_w)$. $x_w$ is called the domain wall (DW) position, and the resulting phase is termed the low density/high density (LD/HD) phase or shock phase (SP), see Fig. S4b.

To find out which of the qualitatively different density profiles (i)–(iii) describes the physical behavior of TASEP/LK with specified parameters, a domain wall analysis has to be performed [5–7]. This essentially amounts to consider a (virtual) DW merging the density functions $\rho_\alpha$ and $\rho_\beta$. The velocity of the DW can be calculated and depending on whether it is (i) positive, (ii) negative, or (iii) vanishes at a position in the lattice bulk, the density profile is given by (i)–(iii) described above.

Here we are interested in the case $\alpha = 0$, cf. Fig. 1b in the main text. As discussed in detail in Refs. [2, 8], only two phases are possible in case $K > 1$: The LD, and the LD/HD phase. In order to distinguish between these profiles, the DW analysis discussed above suggests a simple test: If there is a location $x_w$ on the lattice where $\rho_\alpha(x_w) + \rho_\beta(x_w) = 1$, a domain wall forms at $x_w$ and the full density profile is given in terms of the LD/HD phase. If no such position $x_w$ exists, the LD phase is established.

## S.II. FULL MEAN-FIELD SOLUTION BASED ON TASEP/LK

### A. Reduction to a lattice of constant length

As discussed in the main text, Eqs. (2), the rate of change of MT length and the number of motors on it are given by

$$\partial_t L = \big(\gamma - \rho_+\delta\big)a \ , \tag{S7a}$$

$$\partial_t m = \omega_\mathrm{A}(L/a - m) - \omega_D m - \rho_+\delta \ , \tag{S7b}$$

and $\omega_\mathrm{A}$ and $\gamma$ are given by Eqs. (1) in the main text. This set of equations was complemented by a third equation in the main text, Eq. (4), approximating the flux off the MT, $\rho_+\delta$. In this Section, we will present a more refined theory which invokes an exact solution of Eq. (3) in the main text, and justifies the assumptions made in the main text in more detail.

In Eqs. (S7), the dynamic quantities are $L$, $m$, and $\rho_+$, and $\omega_\mathrm{A}$ and $\gamma$ follow from these equations with Eqs. (1)

in the main text. At stationarity, the fluctuations around $L^*$ and $m^*$ are small, i.e., $\Delta L/L^* \ll 1$, and $\Delta m/m^* \ll 1$. Moreover, the processes changing the length of the MT, or the number of motors on it, are slow compared to the hopping of a single motor. For instance, at a tubulin concentration of $c_T = 2\ \mu$M, even when all tubulin resources are available, the polymerization rate is $\gamma = 0.76\ s^{-1} \ll \nu = 6.35\ \mathrm{s}^{-1}$. Hence, although $L$ and $\omega_\mathrm{A}(m)$ are dynamic quantities, their values are *effectively constant.*

This suggests to reduce our model to an effective model with (exactly) constant attachment rate and (exactly) constant lattice length. Clearly, this is the TASEP/LK, discussed in Sec. S.I, see also Fig. S1. Here, particles attach to the lattice at constant rate $\omega_\mathrm{A}$, independent of the availability of particles, and also the lattice length $L$ is constant. This reduction promises to be a great simplification because TASEP/LK has been studied extensively. In particular, the density profile of particles in this effective model is well known [2], see Sec. S.I.

To ensure that the dynamic and the effective model lead to the same physical observables, we require that

- the TASEP/LK lattice length $L$ equals the (*a priori* unknown) steady state MT length $L^*$, which is determined from the interplay of polymerization and motor-induced depolymerization dynamics,

- the TASEP/LK attachment rate $\omega_\mathrm{A}$ equals the (*a priori* unkown) steady state attachment rate $\omega_\mathrm{A}^* = \omega_\mathrm{A}^0(c_m - m^*/V)$ in the MT model,

- the TASEP/LK detachment rate at the plus end $\beta$ equals the detachment rate from the MT at this site, $\delta$.

Note that because the length of the lattice of TASEP/LK is constant, particle detachment at the plus end (at rate $\beta$) does not change $L$; in addition, no lattice elongation is possible, i.e. $\gamma_0 = 0$ for TASEP/LK.

We can verify the validity of this reduction by comparing the density profiles of motors on the MT with the corresponding profile of particles in TASEP/LK, as they are obtained from simulations. This is shown in Fig. S2. The procedure of calculating the motor density $\rho(x)$ on a lattice of dynamic length is illustrated in Fig. S2e: In order to obtain the density profile in the vicinity of the minus (plus) end of a MT, an ensemble of MTs is aligned along their minus (plus) ends before taking the average; the full density profile is then obtained by merging the two density profiles in the bulk such that the total length of the profile equals the average MT length. As Figs. S2(a)–(d) show for two different sets of parameters, the density profile for the dynamic lattice obtained in this way is in excellent agreement with the corresponding density profiles of the effective TASEP/LK model on a lattice of constant length $L = L^*$ and attachment rate $\omega_\mathrm{A} = \omega_\mathrm{A}^*$.

### B. Strategy to obtain the stationary state

With the reduction of the MT model to TASEP/LK, we can now proceed along the following lines:

(i) In the previous section, Sec. S.II A, we have found that the MT model with dynamic lattice length and resource-limited attachment rate can be reduced to an effective model with constant length and constant attachment rate; the effective model is the TASEP/LK [2].

(ii) For TASEP/LK we know, cf. Sec. S.I and Ref. [1, 2], that there are different phases which have their characteristic particle density profiles. *Assuming* that the system is in one of these phases, we obtain the motor density close to the plus end. Subsequently, mass conservation can be used to obtain an expression for the density $\rho_+$. With the ensuing equation and Eqs. (S7), the steady state quantities $L^*$, $m^*$, and $\rho_+^*$ can be computed.

(iii) Having explicit numerical values for these quantities, it is possible to determine the phase of TASEP/LK with $L = L^*$ and $\omega_\mathrm{A} = \omega_\mathrm{A}(m^*)$. This phase should be the same as the phase which we originally assumed (without specifying parameters) in step (ii). Hence, comparing the *assumed* and the *actual* phase provides a self-consistency check. Given this test is passed, $L^*$ and $m^*$ describe the stationary state.

### C. Case $K > 1$

We will first concentrate on the case $K > 1$, i.e. the case where the motor attachment rate at stationarity exceeds the rate of motor detachment, $\omega_\mathrm{A}^* > \omega_\mathrm{D}$. Because $\alpha = 0$, we know from TASEP/LK [2, 8] that two phases are in principle possible in principle: 1. The LD/HD phase (shock phase), in which the motor densities at the minus and plus end are low and high, respectively, and a domain wall (DW) connects these densities in the MT bulk, and 2. the LD phase, where the density is small along the complete lattice, except for a peak ("spike") at the plus end.

#### *1. Low density/high density (LD/HD) phase*

The simplest case is the LD/HD phase, where the MT becomes stationary at length $L^*_\mathrm{LD/HD}$ with $m^*_\mathrm{LD/HD}$ motors on it. Assuming such a steady state does not imply its existence. Hence, as discussed above, after having found a stationary state, it has to be checked for self-consistency.

In the LD/HD phase of TASEP/LK, the motor density approaches its value at the plus end continuously, see Fig. S4b. Therefore, because $\rho$ varies only slowly with $x$,

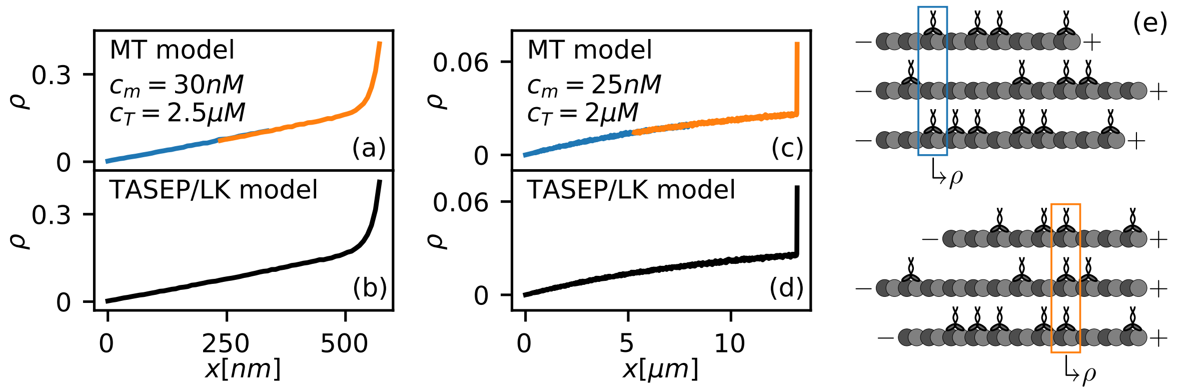


FIG. S2. (a)–(d) Comparison of the occupation density on the MT lattice (top) with the corresponding density of TASEP/LK (bottom). For parts (a) and (c), the concentrations are chosen as in Figs. 2a–2b in the main text, for parts (b) and (d), parameters derive as explained in Sec. S.II A. (e) An ensemble of MTs with a varying length can either be aligned at their minus (top panel), or their plus (bottom panel) ends. The motor occupation density is then obtained by taking the ensemble average, and the full density profile results by merging both averages in the lattice bulk, such that the total length of the profile equals the average lattice length.

the density at the penultimate site (almost) equals the density at the plus end, $\rho_{L-a} \approx \rho_+$. Because of the conservation of the number of motors (mass conservation), the motor current to the tip equals the flux off the MT. We obtain

$$\nu \rho_{L-a}(1-\rho_+) \approx \rho_+ \beta \; , \tag{S8}$$

and hence

$$\rho_{+,\mathrm{LD/HD}} \approx 1 - \beta/\nu \; . \tag{S9}$$

Invoking the correspondence between TASEP/LK and the MT at stationarity, cf. Sec. S.II A, this equation can be used together with Eqs. (S7a) to obtain

$$L^*_{\mathrm{LD/HD}} = aV \left[ c_T - \frac{\delta(1-\delta/\nu)}{\gamma_0} \right] . \tag{S10}$$

In order to be a valid description, $L^*_{\mathrm{LD/HD}}$ obtained in this way should be positive. However, with the model parameters derived in Sec. S.III, we find that $L^*_{\mathrm{LD/HD}} > 0$ only for very large tubulin concentrations, $c_T > 4$ µM, well above the concentration chosen in our *in vitro* experiments. We conclude that the LD/HD phase plays no role for MT length regulation by kinesin motors at our conditions.

### 2. *Low density (LD) phase*

The other phase which is possible for $K > 1$ and $\alpha = 0$ is the low density phase. Here, the motor density remains small along the complete lattice, except for the immediate vicinity of the plus end, where it peaks ("spike"), see Fig. S4a.

In the LD phase, the particle density $\rho(x)$ of TASEP/LK is given by Eqs. (S5a) and (S4). Because the discontinuity at the plus end extends only over very few lattice sites, the density at the foot of the spike (which we denote $\rho_{L-a}$, like in the main text) can be approximated by evaluating the density at position $L$. We therefore obtain

$$\begin{aligned} \rho_{L-a} &\approx \rho_\alpha(L) \\ &= \frac{1}{2}\left\{ \frac{K-1}{K+1} \left[ W_{-1}\big(-Y_\alpha(L)\big) + 1 \right] + 1 \right\} . \end{aligned} \tag{S11}$$

As described in the previous paragraph, the motor current is a slowly varying function of $x$; this is because attachment and detachment are slow compared to the hopping of motors, $\omega_\mathrm{A}, \omega_\mathrm{D} \ll \nu$. Thus, even though the density is discontinuous at the plus end, the motor current is continuous, and hence the current to the tip equals the current off the tip, which implies

$$\nu \rho_{L-2a}[1-\rho_{L-a}] \approx \nu \rho_{L-a}[1-\rho_{L-a}] \approx \rho_+ \beta \; . \tag{S12}$$

Once again invoking the correspondence between TASEP/LK and the MT at stationarity, this results in the expression

$$\rho^*_+ \delta \approx \nu \rho_\alpha(L) \big[ 1 - \rho_\alpha(L) \big] \Big|_{L=L^*, \omega_\mathrm{A}=\omega^*_\mathrm{A}} . \tag{S13}$$

Equation (S13), together with Eqs. (S7) now fully determine all dynamic quantities at stationarity, $L^*$, $m^*$, and $\rho^*_+$. In particular, they define the vector field $(\partial_t m, \partial_t L)$ which we also introduced in the main text, employing a Taylor series solution of $\rho_+ \delta$.

Nonlinear systems of this kind are best analyzed by flow profiles (vector fields) in the phase plane $(m, L)$. The solution of the dynamic equations for $m$ and $L$ can directly be read of as trajectories following stream lines [9]. An example is shown in Fig. S17 for the approximate mean-field solution derived in the main text. For the refined solution of the motor flux off the MT, Eq. (S13), we

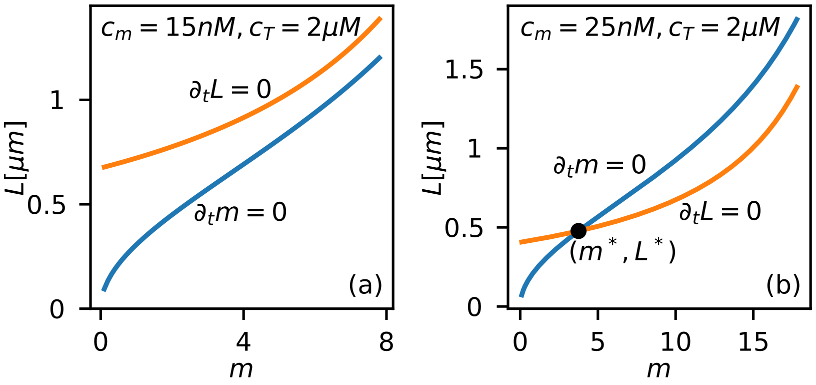


FIG. S3. Nullclines of the vector field $(\partial_t m, \partial_t L)$ for the case $K^* > 1$. As opposed to Fig. S17, here the full mean-field solution for the motor flux off the MT, Eq. (S13), was used. Along the nullclines, $L$ and $m$ become stationary separately. (a) For small motor concentration, $c_m = 15$ nM, we find that $L$ and $m$ do not become stationary simultaneously. Hence, no LD solution with $K^* > 1$ exists for this concentration. (b) For higher motor concentrations, here $c_m = 25$ nM, both nullclines intersect, i.e. the vector field has a fixed point at $(m^*, L^*)$.

have depicted the nullclines of the vector field $(\partial_t m, \partial_t L)$ in Fig. S3. Along the nullclines, the components of the vector field vanish separately, $\partial_t L = 0$ and $\partial_t m = 0$, such that the stationary state, i.e. the fixed point of the vector field, is given by the intersection point of the nullclines. For an exemplary motor concentration $c_m = 15$ nM at $c_T = 2$ $\mu$M, which is depicted in Fig. S3a, no such fixed point exists. This implies that the MT does not have a stationary state in the LD phase for these concentrations. By contrast, for an increased motor concentration $c_m = 25$ nM, Fig. S3b, both nullclines intersect at $(m^*, L^*)$. Hence, a MT with those concentrations may *possibly* become stationary at $m^*$ and $L^*$ in the LD phase.

However, in order to find out whether the MT dynamics will *actually* become stationary at this point, we have to check whether it has been obtained in a self-consistent way. In particular, this implies that two conditions have to be met:

(i) In the derivation of Eq. (S13) we have assumed $K > 1$. Hence, the stationary state described by $L^*$ and $m^*$ should also guarantee $K^* > 1$.

(ii) Furthermore, we have assumed that the TASEP/LK with the (unknown) parameters $L$ and $\omega_\text{A}$ is in the LD phase. Having obtained numerical values, $L = L^*$ and $\omega_\text{A} = \omega_\text{A}(m^*)$, we can now verify whether TASEP/LK with these parameters is actually in the LD phase.

Condition (i) imposes a constraint on the concentration of free, i.e. unbound, motors at stationarity, $c_f^* = c_m - m^*/V$:

$$K^* \overset{!}{>} 1 \Leftrightarrow c_f^* \overset{!}{>} \frac{\omega_\text{D}}{\omega_\text{A}^0} \approx 7 \text{ nM}. \tag{S14}$$

Hence, any steady state which yields a number of motors on the MT, $m^*$, which is so large that the free motor concentration falls below 7 nM, fails to be self-consistent, and must therefore be rejected.

In order to verify the self-consistency condition (ii), we have to analyze in which phase the TASEP/LK with $L = L^*$ and $\omega_\text{A} = \omega_\text{A}(m^*)$ actually is. It is important to understand that the *assumption* of being in the LD phase which lead to Eq. (S13) does not guarantee that the *actual dynamics* of the TASEP/LK is given in terms of this phase! In principle, the phase diagram of TASEP/LK is by now a text book result [2], and thus, given specific motor and tubulin concentrations, and hence specific quantities $L^*$ and $\omega_\text{A}^*$, we could look up the behavior in the phase diagram. However, here we are interested in a general solution. This implies, in analogy with the analysis for TASEP/LK, Sec. S.I, that we have to closely look at the density functions matching the boundary conditions at the minus and plus end, $\rho_\alpha(x)$, and $\rho_\beta(x)$, respectively. We have pointed out in Sec. S.I that if these functions add to 1 at some position $x_w$ on the lattice, a domain wall establishes at this point; the resulting density profile would then indicate a LD/HD phase. Hence, we have to ensure that there is *no such position* $x_w$ on the lattice where the densities $\rho_\alpha(x_w)$ and $\rho_\beta(x_w)$ would add to 1. The procedure of determining whether or whether not a domain wall establishes is illustrated in Fig. S4 for a lattice of (hypothetical) length $L = 100a$. The function $\rho_\alpha(x)$ is a monotonously increasing function. Likewise, provided that the Langmuir density $K/(K+1)$ is smaller than the tip density $1 - \beta/\nu$ which is implied by our simulation results as long as the tubulin concentration $c_T \lessapprox 3$ $\mu$M, the density $\rho_\beta(x)$ is also increasing; this implies that $1 - \rho_\beta(x)$ decreases monotonically with $x$. As $0 = \rho_\alpha(0) < 1 - \rho_\beta(0)$, a condition for the existence of a domain wall at $0 < x_w < L$ is hence $\rho_\alpha(L) > 1 - \rho_\beta(L) = \beta/\nu$. Because the condition for the LD phase is that *no* domain wall exists, a necessary

and sufficient condition for the LD phase is therefore that

$$\rho_\alpha(L) \overset{!}{<} \beta/\nu \ . \tag{S15}$$

Provided this condition is met we have arrived at a self-consistent stationary state.

With the numerical solutions for $L^*$ and $\omega_\mathrm{A}^*$ obtained from Eqs. (S7) and (S13), a numerical test of Eqs. (S14) and (S15) can be performed. In this way, the concentration regime in which the LD phase for $K^* > 1$ yields a physically reasonably, and self-consistent solution, can be constrained, see Fig. 3e in the main text.

### D. Case $K < 1$

In the previous section, Sec. S.II C, we have considered the case of strong motor attachment. Here, we will analyze the opposite case where the motor concentration is either so small or so strongly depleted in the cytosol that at stationarity $\omega_\mathrm{A}^* < \omega_\mathrm{D}$. In the effective model, the TASEP/LK, to which we have reduced the length regulation model of a MT, see Sec. S.II A, this corresponds to the case $K < 1$. For this case, the density profiles of particles on the lattice are most easily obtained by using the particle-hole symmetry of TASEP/LK: Here, instead of considering the motion of motor particles to the right, we may look at the motion of holes, i.e. lattice sites with *no* motors on them, moving to the left [2]. In this picture, particle attachment corresponds to hole detachment and motor detachment to hole attachment. As a consequence, the concentration-limited process is *detachment* of holes. Having arrived at the left lattice end, holes exit the lattice at the same rate as particles enter at this site; likewise hole injection at the plus end corresponds to motor detachment from this site.

In conclusion, denoting the hole parameters and coordinates with a bar, we therefore employ the following correspondence of TASEP/LK and the dynamic MT at $K < 1$:

$$\begin{aligned}
&\overline{L} = L = L^*, \quad \overline{x} = \overline{L} - x, \quad \overline{\rho} = 1 - \rho, \\
&\overline{\nu} = \nu, \quad \overline{\alpha} = \beta = \delta, \quad \overline{\delta} = \alpha = 0, \\
&\overline{\omega_\mathrm{A}} = \omega_\mathrm{D}, \quad \overline{\omega_\mathrm{D}} = \omega_\mathrm{A} = \omega_\mathrm{A}^* = \omega_\mathrm{A}^0(c_m - m^*/V) \ .
\end{aligned} \tag{S16}$$

With this symmetry mapping, we can now proceed along the same lines as before. In Sec. S.II C we concluded that in the specific case $\alpha = 0$ at $K > 1$ two phases, the LD and LD/HD phase are possible. Similarly, for $K < 1$ where $\alpha = 0$ implies $\overline{\delta} = 0$ in the hole picture, we find that only two phases are possible which we will call low hole density/high hole density (LhD/HhD) phase, and low hole density (LhD) phase in the following. For the former, the hole density is small around the injection site of holes (i.e., at the MT plus end), and a DW in the lattice bulk connects this density to the high hole density at the opposite end (the minus end). In terms of the particle density, this implies a very similar density profile as for the LD/HD phase, Sec. S.II C 1.

For the other phase which is possible in this case, the high hole density (HhD) phase, the hole density is high (i.e., the motor density is small) along the complete MT, except for a small boundary layer at the hole injection (i.e., the motor exit) site.

#### 1. *Low hole density/high hole density (LhD/HhD) phase*

In the first case, where the hole density profile on the lattice is low at the injection site and high at the other end, and a DW separates these regions on the lattice, we can directly use the results of Sec. S.II C 1: Here, we made use of the fact that if a domain wall forms in the lattice bulk, the density is continuous at both ends, which lead to an equation for the motor density at the plus end, Eq. (S9). Since the same is true for the LhD/HhD phase, we find that the stationary state length is also given by Eq. (S10). However, since we concluded earlier that the tubulin concentration would have to exceed 4 $\mu$M such that this steady state length would be positive, we find that also in the case of weak motor attachment, $K^* < 1$, no stationary state showing a domain wall will be observed for conditions of our *in vitro* experiments.

#### 2. *High hole density (HhD) phase*

The only remaining phase is characterized by a high hole density (i.e., low motor density) along the complete MT. Similar to the LD phase, Sec. S.II C 2, the hole density is discontinuous at the plus end of the lattice, where holes are injected, i.e., at $\overline{x} = 0$.

In full analogy with the case $K > 1$, from the notion that the flux of holes (and thus also the flux of motors) is constant on short length scales, we now conclude that the motor flux off the MT equals the hole flux onto the lattice, which equals the hole current a small distance away from the tip. In accordance with Eq. (S13), this yields

$$\rho_+^* \delta = \overline{\nu} \overline{\rho}_{\overline{\delta}}(0) \left[1 - \overline{\rho}_{\overline{\delta}}(0)\right] \Big|_{\overline{L}=L^*, \overline{\omega_\mathrm{D}}=\omega_\mathrm{A}^*, \overline{\delta}=\alpha=0, \overline{\nu}=\nu} \ . \tag{S17}$$

In the same way as discussed in Sec. S.II C 2, Eq. (S17) together with Eqs. (S7) defines a vector field $(\partial_t m, \partial_t L)$, whose fixed points define the stationary quantities $L^*$ and $m^*$.

These fixed points have to be checked for self-consistency. In analogy with Sec. S.II C 2, this amounts to ensure that no position $\overline{x_w}$ exists where the two density solutions matching the respective boundary conditions, $\overline{\rho}_{\overline{\alpha}}(x)$ and $\overline{\rho}_{\overline{\delta}}(x)$, would add to 1, i.e. $\overline{\rho}_{\overline{\alpha}}(\overline{x_w}) = 1 - \overline{\rho}_{\overline{\delta}}(\overline{x_w})$. Because we know that $1 - \overline{\rho}_{\overline{\delta}}(\overline{L}) = \rho_\alpha(0) = 0 < \overline{\rho}_{\overline{\alpha}}(\overline{L})$, it is sufficient to compare the hole density at the site where they are injected, i.e. at the MT's plus end:

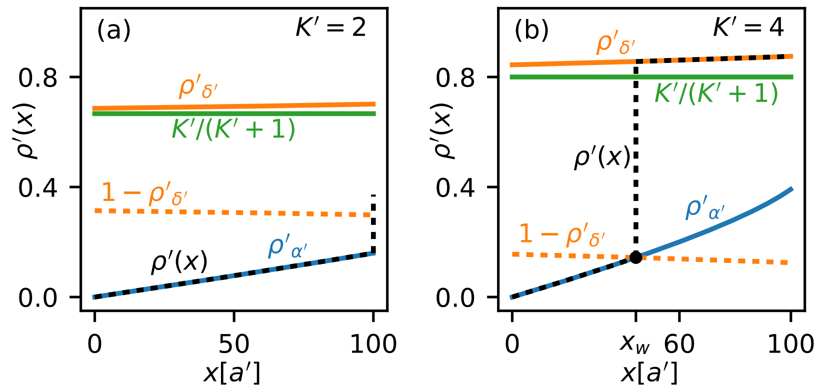


FIG. S4. Construction of the full density profile of TASEP/LK, and distinction between the LD, and LD/HD phase. Shown are the density functions $\rho_\alpha(x)$ and $\rho_\beta(x)$ for a (hypothetical) lattice length $L = 100a$, for two different values of $K$. In both cases, the $\beta$ branch of the density profile lies above the Langmuir density $K/(K+1)$, which implies that the density function $\rho_\beta(x)$ increases monotonically [2]. In part (a), which shows an exemplary profile of the LD phase, at no position along the lattice the density functions $\rho_\alpha$ and $\rho_\beta$ add to 1, i.e., $\rho_\alpha$ and $1-\rho_\beta$ do not intersect. This implies that no domain wall forms at these conditions. The full density profile $\rho(x)$ for this case is therefore identical to the branch $\rho_\alpha(x)$, and the density shows a discontinuity at the plus end, such that $\rho_\alpha(L)(1-\rho_\alpha(L)) = \rho_+\beta$. For the conditions shown in part (b), exemplary for the LD/HD phase, the behavior is different: Here, a DW is localized at position $x_w$, where $\rho_\alpha(x_w) + \rho_\beta(x_w) = 1$. Therefore the full density profile is given by $\rho_\alpha(x)$ for $x < x_w$ and $\rho_\beta(x)$ for $x > x_w$, as indicated by the black dotted line.

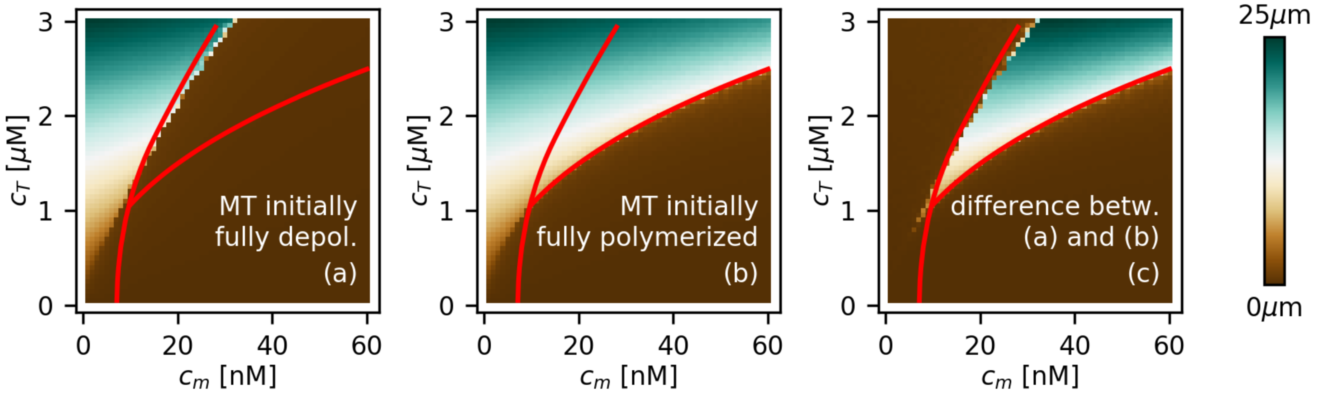


FIG. S5. Parameter scan of the motor and tubulin concentrations for a lattice which is initially short, part (a), or long (b). The color code indicates the stationary MT length, cf. also Fig. 3a–3b in the main text. Red lines show the phase transition lines obtained from the full mean-field theory, Sec. S.II. Part (c) shows the difference of the first two panels, and reveals that the theoretical phase transition lines indeed constrain the bistable regime, see also Fig. 3e in the main text.

If $1-\overline{\rho}_{\overline{\delta}}(0) < \overline{\rho}_{\overline{\alpha}}(\overline{L}) = 1-[1-\rho_\beta(L)] = \beta/\nu$, no domain wall can localize on the lattice. In this case, the solutions obtained from Eqs. (S17) and (S7) are self-consistent.

### E. Comparison with simulations, and the phase diagram/stability diagram

Having completed the mean-field analysis, we are now in a position to compare these analytical results with simulation data. Fig. 3d in the main text shows the MT length as a function of the motor concentration $c_m$ at $c_T = 2$ μM. Mean-field theory and simulations show excellent agreement. Starting at low motor density, the stationary length is long (i.e., polymerization dominates), and $K^* < 1$. At high motor densities, the steady state length is short (depolymerization dominates) with $K^* > 1$. In the bistable regime for intermediate concentrations, a third solution exists which connects the two branches. We have discussed in the main text that this solution is unstable, and we can obtain its numerical value from the full mean-field theory as a solution of the HhD phase in case $K^* < 1$, Sec. S.II D 2.

We can use the self-consistency conditions together with the steady state solutions obtained in the previous sections to summarize the domains in which $K^* > 1$ and $K^* < 1$, respectively, see Fig. 3e in the main text. As expected from simulations, the two regimes overlap; in

the overlapping part, length regulation is bistable. with simulation data, Figs. 3a and 3b in the main text, reveals that the steady state MT length obtained in simulations starting from a short and long length, respectively, changes discontinuously at the respective transition lines; this is because the phase transition lines describe the onset (and offset) of bistability. This is also illustrated in Fig. S5c which shows the difference of $L^*$ obtained in simulations starting from long, and short length, respectively.

In conclusion, the mean-field theory developed in this Section is in excellent agreement with simulation data.

## S.III. ESTIMATION OF THE PARAMETERS

We are interested in a theoretical description of the motion of the molecular motor Kip3 on MTs. For many of the motility parameters, accurate measurements exist which allow us to assign numerical values to most parameters. We have summarized all parameters in Table. S.I and will show how to obtain their values in this Section.

Kip3 motors move at 3.2 $\mu$m/ min [10]. In units of the distance between two tubulin dimers $a = 8.4$ nm [11], this gives rise to the hopping rate to the neighboring lattice site, $\nu = 6.35$ sites/s.

Kip3 runs on the MT for 11 $\mu$m [10] at this speed, i.e., their dwell time is 206 s. Taking the inverse, this yields the detachment rate $\omega_{\rm D} = 4.9 \cdot 10^{-3}$ s$^{-1}$. The run length might be an underestimate, but the specific value of $\omega_D$ is relatively unimportant, as long as it is small.

In order to obtain the spontaneous polymerization rate of MTs, we consider the polymerization speed of stabilized MTs (these are MTs in which the GTP analogue GMP-CPP is used to grow MTs in order to avoid dynamic instability) which we have used in our *in vitro* experiments [12, 13]. Hyman et al. [12] measured the speed of MT growth, and find the value 0.19 $\mu$m min$^{-1}$ $\mu$M$^{-1}$, corresponding to a dimer polymerization rate of $\gamma_0 = 0.38$ $\mu$M$^{-1}s^{-1}$ on each protofilament. The same value was obtained by Brouhard et al. [13]. Here, we neglect (slow) spontaneous MT depolymerization (which was measured to be as low as 0.23 $\mu$m/$h$ [12], which corresponds to a spontaneous tubulin loss rate of $7.6 \cdot 10^{-3}$ s$^{-1}$ on each protofilament; another study [13] indicates a slightly higher tubulin loss rate per protofilament of $3.8 \cdot 10^{-2}$ s$^{-1}$, which is still small). A recent study has indicated that the tubulin exchange rate at the MT tip is indeed much faster than reported previously [14]. However, the net spontaneous polymerization in this study, i.e. the difference of spontaneous polymerization and depolymerization is comparable to the values reported by Hyman et al. [12] and Brouhard et al. [13]. Since we are only interested in the net values, the estimates of these studies therefore remain valid for our purposes.

The attachment rate of Kip3 motors to a binding site on a MT can be obtained from the motor landing rate measured per concentration, per time, and per length, for which Varga et al. obtained the value 24 nM$^{-1}$min$^{-1}\mu$m$^{-1}$ [10]. The interpretation of this value is not straightforward for two reasons: Firstly, the landing rate critically depends on the number of motors which are already attached to the MT, and even at smalls motor concentration it may be significantly depleted due to a reduced availability of binding sites [15]. Secondly, it is not clear how to convert a per-$\mu$m attachment rate to a per-site attachment rate: The measurement of Varga et al. [10] was done in a TIRF setup, where motors can probably bind to and walk on roughly 5 protofilaments (the "upper half") [16]. We decided to use the resulting $5 \cdot 1000/8.4$ binding sites as the conversion factor between the per-$\mu$m and the per-site attachment rate. This results in the per-site attachment rate $\omega_{\rm A}^0 = 6.7 \cdot 10^{-4}$ nM$^{-1}$s$^{-1}$.

For the depolymerization process, we note that the mechanism of Kip3 induced MT depolymerization is not fully understood. However, we can obtain a lower bound for $\delta$ from the MT depolymerization speed at high kinesin concentration, which is $\sim 1800$ dimers/min (counting all protofilaments) [10]. Therefore, the lower bound for the dimer depolymerization rate per protofilament is $\delta \approx 2.3$ s$^{-1}$.

The volume $V$ from which protein can bind to the MT, i.e. the "basin" of a MT, is difficult to measure directly. We find in experiments that for MTs grown for 1.5 or 3 hours, between 35% and 40% of all tubulin is incorporated into the MTs, see Fig. S16. At these times of incubations, MTs were on average 4.8 $\mu$m and 10.8 $\mu$m long, respectively, Fig. S20. This implies that between 1,600 and 3,200 tubulin dimers are available for each protofilament [17]. Here, we are mostly interested in a rough estimate of the effective volume. Therefore we chose $V$ in a way convenient for our simulations, such that a tubulin concentration of 2 $\mu$M, typical for experiments, corresponds to 2,000 tubulin heterodimers available per protofilament. The resulting effective volume per protofilament is $V = 1.66$ $\mu$m$^3$. We also verified that the particular choice of $V$ plays no essential role for the phenomena, see Sec. S.IV and Figs. S9–S14.

## S.IV. ROBUSTNESS OF THE PARAMETERS $\delta$ AND $V$

Here we test our model for robustness against variations of its parameters. In particular, the values of the depolymerization rate $\delta$ and the volume available to each protofilament, $V$, have quite significant uncertainties. We have varied these parameters in Figs. S9–S14. These Figures show a parameter scan of the motor and tubulin concentrations, starting from a short, or long length, see also Figs. 3a–3b in the main text. In particular, parts (c) of these Figures shows the difference of the simulation results obtained in panels (a) and (b), and hence indicate the concentration regimes in which length regulation is bistable.

We find that the precise value of $\delta$, of which 2.3 $s^{-1}$

| quantity | symbol | value | reference |
|---|---|---|---|
| hopping rate | $\nu$ | $6.35\ \mathrm{s}^{-1}$ | [10] |
| MT lattice spacing | $a$ | 8.4 nm | [11] |
| detachment rate | $\omega_\mathrm{D}$ | $4.9 \cdot 10^{-3}\mathrm{s}^{-1}$ | [10] |
| attachment rate per site | $\omega_\mathrm{A}^0$ | $6.7 \cdot 10^{-4}\ \mathrm{nM}^{-1}\mathrm{s}^{-1}$ | [10] |
| polymerization rate | $\gamma_0$ | $0.38\ \mu\mathrm{M}^{-1}\mathrm{s}^{-1}$ | [12, 13] |
| depolymerization rate | $\delta$ | $2.3\mathrm{s}^{-1}$ | [10] |
| volume avail. per protofil. | $V$ | $1.66\ \mu\mathrm{m}^3$ | estimated |

TABLE S.I. Overview of the model parameters, as obtained in Sec. S.III

is a lower bound, has no effect on the resulting stability diagram (phase diagram), when its value is increased threefold. In contrast, the volume per protofilament $V$, has a mild effect: When it is increased, the region in which MT length regulation is bistable, i.e. where the MT length may assume one of two stationary states, becomes larger. However, the general qualitative behavior remains unaltered.

The observation that the concentration regime for bistable length regulation becomes smaller for smaller basin volume $V$ suggests an additional and alternative interpretation why the MT length distribution is unimodal for MTs grown for 1.5 hours only, and bimodal for MTs grown for 3 hours, see the main text and Figs. S15a and 4a. If, for any reason, the MT density in solution was larger for the shorter set of experiments, i.e., the volume available for each MT was smaller, the expected concentration regime in which MT length is bistable would also have been smaller. Then, it is in principle possible, that the relatively coarse sampling of length distributions at motor concentrations 0 nM, 4 nM, 20 nM, and 400 nM, has completely misses the bistable domain. In fact, the number of MTs counted per channel was larger for the set of experiments where MTs had been grown for 1.5 hours before addition of Kip3, Fig. S15b, than for the 3 hours experiments, Fig. 4b. This could indicate a higher MT density in solution, but could also be the result of fluctuations of the antibody density in the channels. At present, we are unable to distinguish between these two interpretations. Both of them are possible within our theoretical analysis. Future studies will help to distinguish between them, and will enable us to more closely investigate the role of the volume available to each MT.

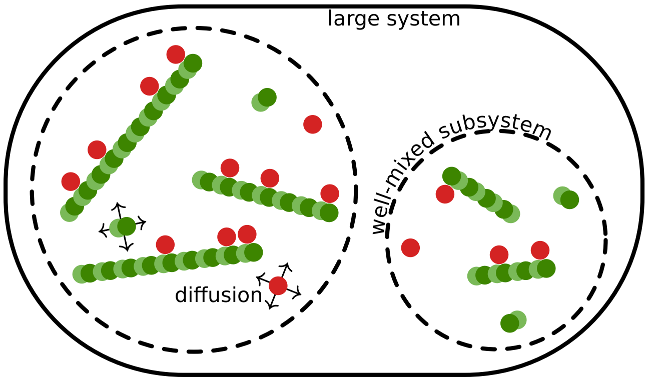


FIG. S6. A large system with many MTs which share common pools of resources. Tubulin and molecular motors can be exchanged between the MTs via diffusion. Here, the spatial arrangement of MTs becomes important: Diffusion can lead to quick exchange of resources on a local scale while it is slow on long length scales. Hence, we may decompose the large system into smaller parts: Within these subsystems, resources are well-mixed, whereas two subsystem behave independently.

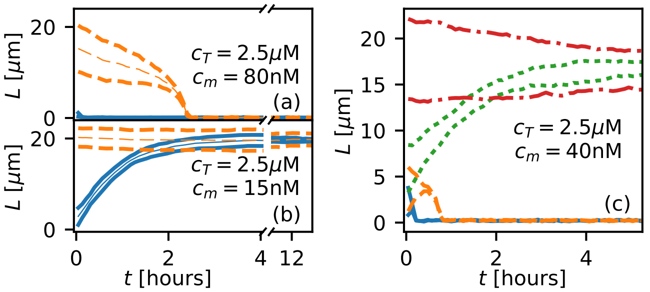


FIG. S7. Simulation runs of a system of two MTs sharing a common pool of resources. Different colors represent different simulation runs, whereas a common color is used for the two MTs of a specific run. In parts (a)–(b), concentrations are chosen such that the dynamics are in the monostable regime. Even if the individual length (thick lines) of the two lattices is very different initially, they approach the same value at the stationary state. Hereby, equilibration is faster for the average length (thin lines) than for the length of individual filaments. Because the dynamics are monostable, the MTs in all simulation runs evolve towards a single stationary length which may be (a) short, or (b) long. Panel (c) shows trajectories for concentrations in the bistable regime. Here, both MTs of each simulation run approach the same steady state; the joint stationary length may be either short or long. Therefore, also a two-MT system shows bistability. Which of these stationary states is reached depends on the initial average length of the MTs.

## S.V. MANY MTS WITH SHARED RESERVOIRS

So far, we have considered a model with only a single MT which has exclusive access to a reservoir of protein. However, inside a cell, as well as in our *in vitro* experiments, many MTs compete for a pool of tubulin dimers and molecular motors which is shared between all MTs. Fig. S6 shows such a system schematically, and it illustrates the additional complexity which arises in such a system: While the motion of motors along MTs happens in a directed fashion, protein exchange between the filaments is only possible via diffusion. Already for a single MT, the consideration of diffusion significantly complicates a theoretical treatment [18]. With many MTs in a system, diffusion furthermore leads to an additional spatial component, which eventually demands that the three-dimensional arrangement of the MTs in the system is specified. A model like this is highly interesting and can lead to emergent phenomena [19, 20], but it is far beyond the scope of this work.

Instead, here we want to focus on a simplified model, making use of a separation of length scales. On short length scales, diffusion is fast, so that on these scales, the system can be assumed to be well-mixed: There, all components are shared infinitely fast. In contrast, on longer length scales, diffusion is slow, so that distant MTs develop independent of another. This suggests to decompose our large system into smaller independent, well-mixed subsystems, see Fig. S6: Inside a subsystem, diffusion is assumed to be infinitely fast, whereas no resource exchange takes place between subsystems. We will later argue the implications of this kind of separation, and indicate how our results can be connected to an *in vitro* or *in vivo* system.

### A. Shared reservoirs with infinitely fast diffusion

Let us first focus on the case of several MTs in a small subsystem which is assumed to be well-mixed. This is the opposite limit compared to the model of a single, isolated MT, considered in the main text. More specifically, we consider the case of two MTs which share a common pool of resources which are exchanged between filaments infinitely fast. To compare with the original model, Fig. 1b in the main text, we have chosen all parameters of the many-MT model equal to those of the single-MT model, and the volume of the system is doubled, such that the effective volume available per MT remains the same. Figure S7 shows trajectories of the length of the two filaments at different conditions. For two sets of concentrations, Figs. S7a–S7b reveal that the length of both MTs assumes a common value relatively quickly. At these conditions, the stationary state is reached independent of the initial MT lengths. For the concentrations shown in these Figures, the dynamics are therefore monostable.

In contrast, for the concentrations used in Fig. S7c, length regulation is bistable. Here, we find that the length of both MTs of a single simulation run still approach the same value. However, depending on the initial conditions, this length may be either short, or long. In particular, our simulation results indicate that when the average initial length of the two MTs is relatively short, it is likely that both MTs will evolve towards the

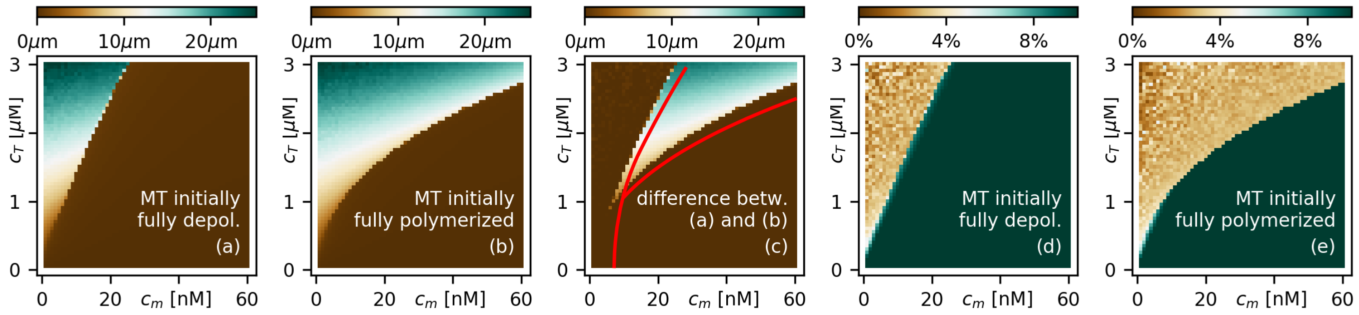


FIG. S8. Scan through motor and tubulin concentrations for a system of two MTs sharing a common pool of resources. Simulation results show the MT length starting from an initially (a) short and (b) long lattice. Part (c) shows the difference of the steady state length obtained in this way, and compares the resulting bistable regime with the results obtained theoretically for the single-MT model (red line). (d)–(e) show the relative standard deviation of the length of the two MTs, averaged over time, see Eq. (S20). In the regime where MT are not completely depolymerized at stationarity (i.e., in the North West part of the Figure), the relative deviation remains small. In the South East region, MTs are very short; although the relative deviation is large here, the absolute standard deviation of both MT lengths is therefore small. This proves that the length of both MTs is very similar.

fixed point with short length. By contrast, for initially (on average) long MTs, the long length will be reached. We conclude that bistability is found also when two (or more) MTs share a common pool of resources infinitely fast, but that all MTs in a well-mixed system of this kind approach the same stationary length.

Let us provide a theoretical argument why, even in the case of bistability, all MTs in the system share the same length. The balance equations, describing the rate of change of MT length and the number of motors on it, Eqs. (2) in the main text, can be straightforwardly generalized to many MTs:

$$\partial_t L^i = \left(\gamma^i - \rho_+^i \delta\right) a \ , \tag{S18a}$$

$$\partial_t m^i = -\omega_\mathrm{D} m^i + \omega_\mathrm{A}^i (L^i/a - m^i) - \rho_+^i \delta \ , \tag{S18b}$$

where the superscript $i$ indicates that these equations apply to all of the $N$ MTs in the system. Assuming that components in the cytosol are instantaneously available for any MT, the polymerization rate $\gamma^i$, as well as the attachment rate of motors to the MT, $\omega_\mathrm{A}^i$, depend only on the *global* availability of protein:

$$\gamma^i = \gamma = \gamma^0 \left[c_T - \sum_i L^i/(aV)\right] \ , \tag{S19a}$$

$$\omega_\mathrm{A}^i = \omega_\mathrm{A} = \omega_\mathrm{A}^0 \left(c_m - \sum_i m^i/V\right) \ . \tag{S19b}$$

These equations imply that when, e.g., a tubulin dimer attaches to any of the $N$ MTs and therefore elongates it, this will have the same immediate effect on the polymerization rate of all MTs. To explore the consequences of infinitely fast resource sharing, let us consider the rate of change of the length of a MT, Eq. (S18a). With Eqs. (S19), we find that $\gamma^i$ is equal for all MTs, such that in the stationary state, when $\partial_t L^i = 0$, also the plus end density must be the same for all lattices, $\rho_+^i = \rho_+$. $\rho_+$ is determined from the balance of currents: The bulk current to the tip equals the motor flux from the tip. We concluded in Sec. S.II that for relatively small motor concentrations, as considered in this work, the motor density remains small along the complete MT. From Ref. [2] we know that for this case both the motor density and their current increase with distance from the minus end. The lattice therefore acts as an antenna, and the longer it is the more motors it can attract. As a consequence, the density of motors at the tip is monotonously increasing with MT length. With Eq. (S18a) we therefore obtain that the MT length is equal for all MT in the system, $L^i = L$.

In order to examine how the concentration regime in which the system behaves bistable is modulated in a two-MT system compared to a single MT, we have performed a scan through motor and tubulin concentrations analogous to the single-MT model (Fig. 3a–3b in the main text). The resulting diagrams are shown in Fig. S8. In Fig. S8a, the average length of the two MTs is shown when simulations start from a short length, in Fig. S8b simulations begin at a long MT length. Fig. S8c shows the difference of these states' stationary length. We find that this difference is large in an extended parameter region; here, two distinct stationary states exist: MT length regulation is bistable is the domain. Fig. S8c also compares the extension of the bistable regime for a system of two well-mixed MTs (color code) with the result obtained for a single MT (red line), cf. Fig. 3e in the main text.

Furthermore, with the help of simulations, it is possible to systematically explore how accurate length regulation of the individual MTs functions. To this end, we have computed the deviation of the MTs' length from their average. We denote with $\overline{L}_t$ the momentary average length of the two MTs at time $t$. A good measure for the accuracy of length regulation is the average relative

standard deviation of MT length,

$$\left\langle \frac{\sqrt{\sum_i (L_i - \overline{L}_t)^2}}{\overline{L}_t} \right\rangle_t . \tag{S20}$$

Here, $\langle \cdot \rangle_t$ signifies that the average is taken over time. This quantity is depicted in Figs. S8d–S8e. We observe that for small motor concentrations and large tubulin concentrations (the North West part of these diagrams), the relative deviation of the MTs' length from their average value is small. For large motor, or small tubulin concentrations (the South East part), the relative deviation is large. However, we find that the concentration regime confined in this way is identical to the domain in which the MTs completely depolymerize, Figs. S8a–S8b. Therefore, absolute fluctuations are small in this domain. In conclusion, length regulation functions accurately for all concentrations.

Taken together, when resources are shared infinitely fast between two or more MTs, we recover the findings obtained for a single MT. The length regulatory mechanism is accurate, and bistability also persists in these larger systems.

### B. Shared reservoirs with finite diffusion

Having discussed the case of many MTs in a well-mixed system, let us now examine the implications of these findings for an *in vitro* or *in vivo* experimental system.

First, let us estimate when the assumption of a well-mixed system breaks down. With Fick's law, typical diffusion constants of several $10^{-8}\text{cm}^2\text{s}^{-1}$ [21] for tubulin imply that within the time it takes for MTs to reach their stationary length, say, an hour (Fig. S7), the length scale which is explored by free diffusion is of the order of several 100 $\mu$m. This is significantly below the length scales of our experimental setup. Therefore, in the *in vitro* experiments performed in this study, it is likely that the global system does not behave well-mixed but rather that different parts of the solution may develop independently.

We found in the previous Section that MTs in a well-mixed system can either become short, or long, but all of these MTs approach the same length. In spatially separated regions, MTs can therefore evolve differently: If the local average initial length in a part of system is short, the MTs in this region is likely to evolve collectively towards the short length; if in another part the initial local average length is long, these MTs will get long. Therefore, patches of long and short MTs will emerge which are spatially separated. In conclusion, when the length distribution of the resulting population of MTs is measured under a microscope, we expect two "classes" of MTs: One class of short, another with long length. This is what we find in our *in vitro* experiments: In a certain concentration regime, MTs with two characteristic length scales coexist, Fig. 4a. Further evidence for the existence of spatial patches comes from an experiment, where Kip3 was added to MTs at a concentration of 20 nM, and one part of the solution was incubated at rest, whereas the other part was mixed constantly. In the latter case, we expect that the complete system may be considered well-mixed. Therefore, it is unlikely that spatial patches of different tubulin length exist. In fact, in the case of constant mixing, the length distribution of MTs is unimodal, as opposed to the bimodal distributions for MTs at rest, Fig. S18. We conclude that bistability in the sense of our theoretical treatment imply bimodal length distributions in our *in vitro* experiments.

Whether bistable length regulation, and the associated two classes of MTs, as described in this work becomes important in cells, we may not say with certainty. On one hand, length scales, e.g. in the mitotic spindle [22, 23] are shorter than the extension of our experiment. As a consequence, one might think that in a system like a cell, protein is well-mixed. On the other hand, protein cannot diffuse freely within a cell due to the presence of intracellular structures such as cytoskeletal filaments. It is likely that under these crowded conditions, diffusion is significantly slowed down. In addition, both kinesin and tubulin can associate with MTs. If, for example, a kinesin-8 motor attaches to a MT, it may remain there for minutes and longer, because the detachment rate from the MT is very small [10], and the motor typically has to walk until the end of the MT until it may detach [24]. In conclusion, we hypothesize that the separation of length scales, such as described here, is also relevant in cells. Hence, also here, we expect that bistability and the associated two distinct classes of MTs are important.

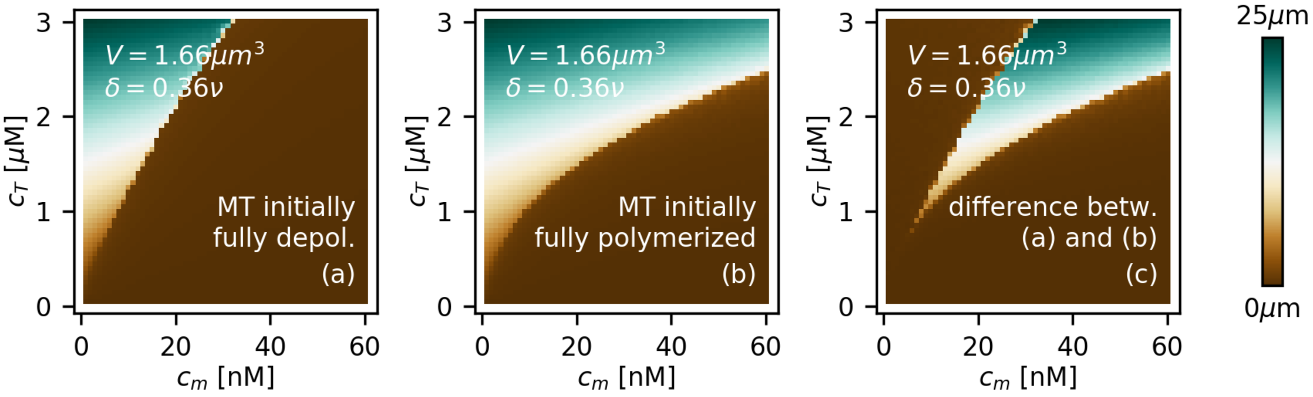


FIG. S9. Scan of the MT length (color code) with the motor and tubulin concentrations as control parameters, see also Figs. 3a–3b in the main text. In panel (a), MTs are initially short, in panel (b), MTs start fully polymerized. Part (c) shows the difference between the values obtained in the first two parts, and therefore indicates the parameter regime in which MT length is bistable. Because the estimates for the volume $V$ and the depolymerization rate $\delta$ have significant uncertainties, we explore in which way the dynamics change when these parameters are varied. Here, $\delta = 2.4\ \mathrm{s}^{-1} = 0.36\nu$, $V = 1.66\mu\mathrm{m}^3$ (such that 1 $\mu$M$\hat{=}$1000 dimers per protofilament).

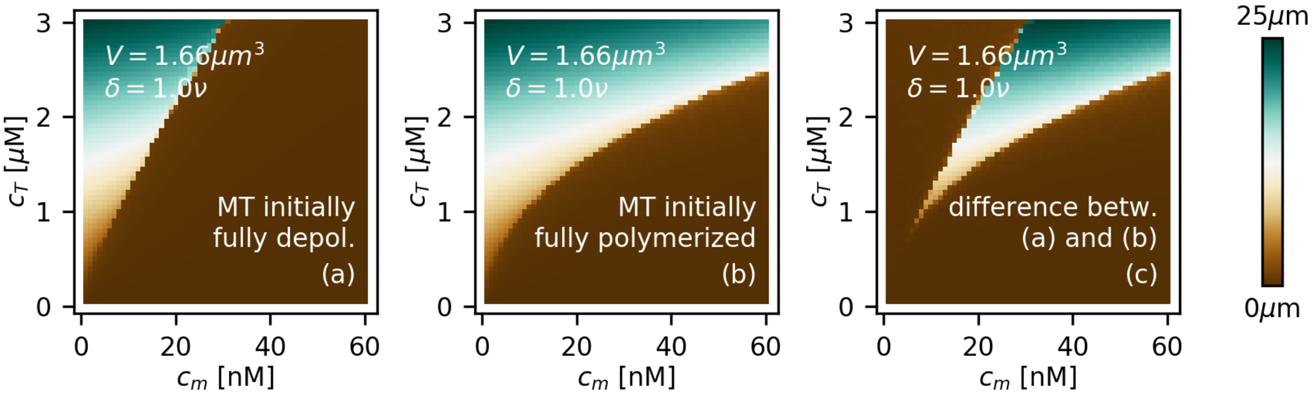


FIG. S10. As in Fig. S9, but with $\delta = 6.35\ \mathrm{s}^{-1} = \nu$, $V = 1.66\mu\mathrm{m}^3$ (such that 1 $\mu$M$\hat{=}$1000 dimers per protofilament).

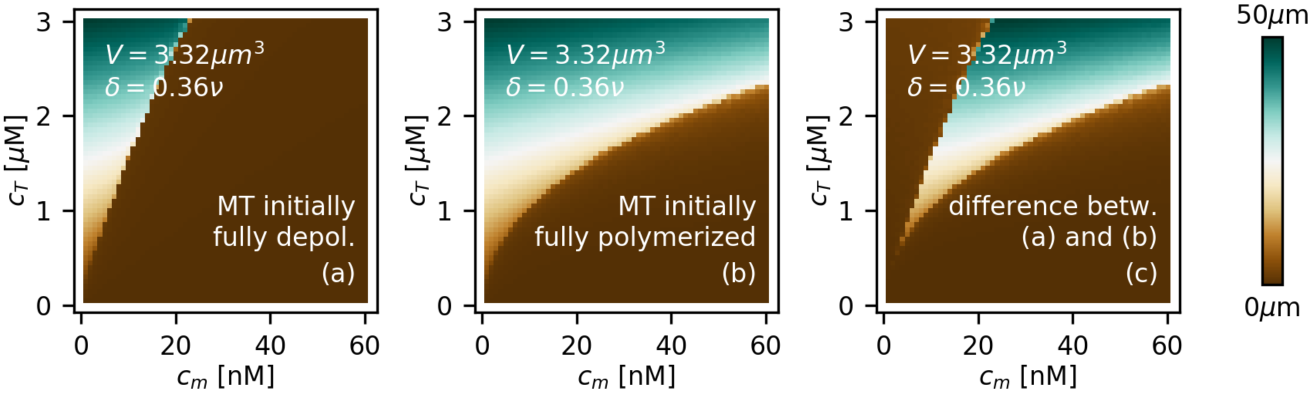


FIG. S11. As in Fig. S9, but with $\delta = 2.4\ \mathrm{s}^{-1} = 0.36\nu$, $V = 3.32\mu\mathrm{m}^3$ (such that 1 $\mu$M$\hat{=}$2000 dimers per protofilament).

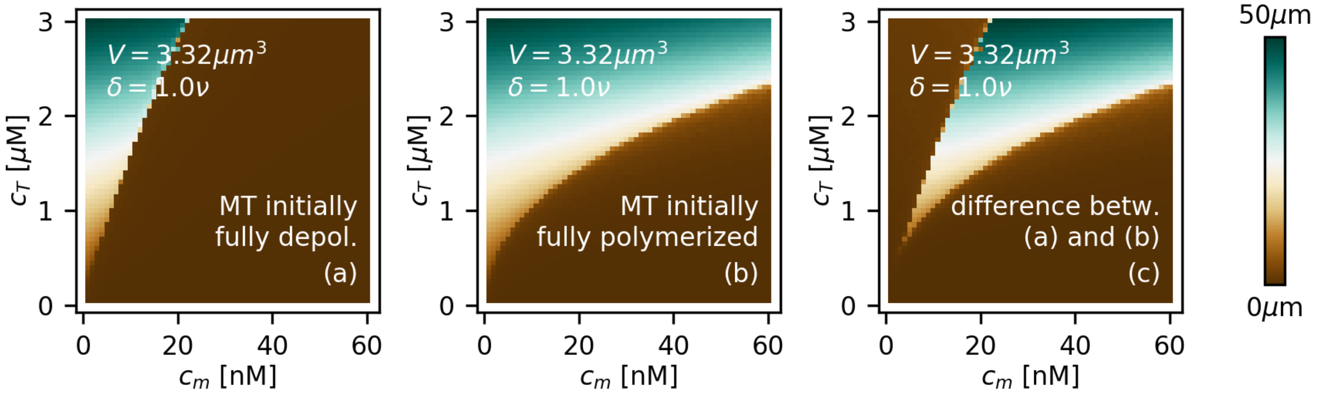


FIG. S12. As in Fig. S9, but with $\delta = 6.35\ \mathrm{s}^{-1} = \nu$, $V = 3.32\mu\mathrm{m}^3$ (such that 1 $\mu$M$\hat{=}$2000 dimers per protofilament).

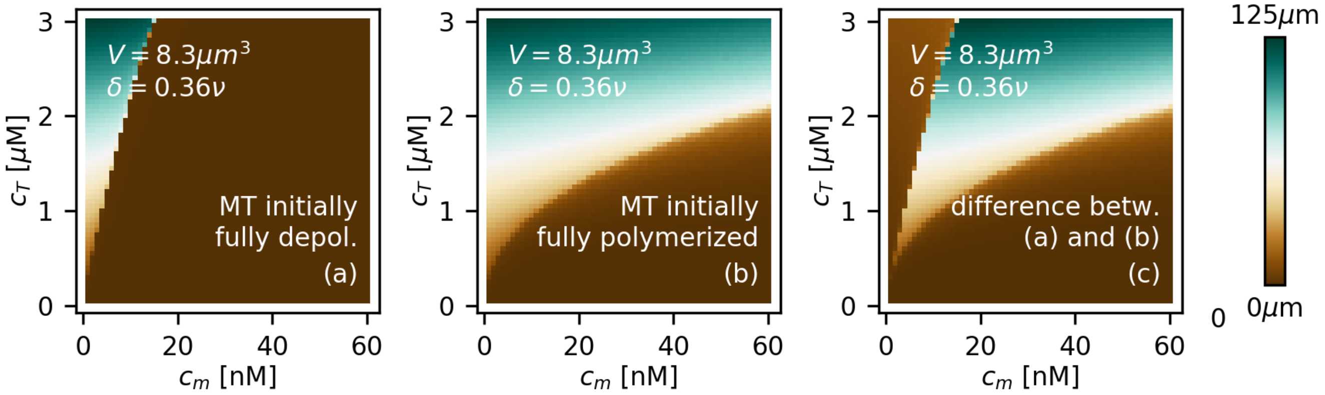


FIG. S13. As in Fig. S9, but with $\delta = 2.4\ \mathrm{s}^{-1} = 0.36\nu$, $V = 8.3\mu\mathrm{m}^3$ (such that 1 $\mu$M$\hat{=}$5000 dimers per protofilament).

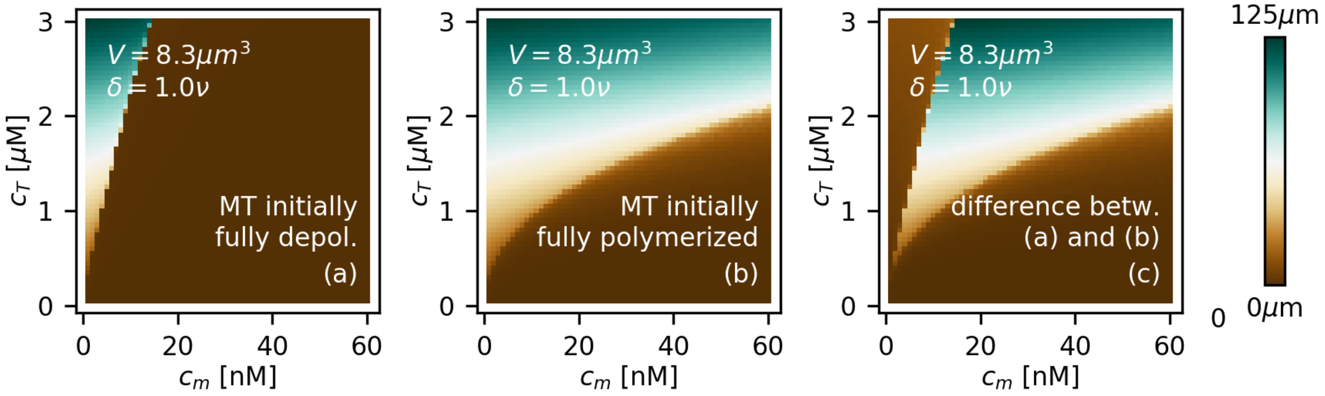


FIG. S14. As in Fig. S9, but with $\delta = 6.35\ \mathrm{s}^{-1} = \nu$, $V = 8.3\mu\mathrm{m}^3$ (such that 1 $\mu$M$\hat{=}$5000 dimers per protofilament).

## S.VI. EXPERIMENTAL METHODS

*a. Protein expression and purification.* Porcine tubulin was purified from porcine brain (Vorwerk Podemus, Dresden, Germany) using established protocols as described previously [25]. Histidine-eGFP tagged *Saccharomyces cerevisiae* kinesin-8, Kip3-eGFP, was expressed and purified using established protocols as described previously [26].

*b. MT polymerization.* To produce GMP-CCP grown rhodamine labeled MTs, a MT polymerization (MTP) solution was incubated on ice for 5 minutes and then for 1-3 hours (duration determines the MT length distribution) at 27 °C to polymerize MTs. The MTP solution consisted of 100 $\mu$l of BRB80 (80 mM Pipes [Sigma], pH 6.9, with KOH [VWR], 1 mM EGTA [Sigma], 1 mM MgCl2 [VWR]) supplemented with 2 $\mu$M porcine tubulin (1:3 mixture of rhodamine-labeled and unlabeled), 1 mM GMP-CPP (Jena Bioscience, Jena, Germany) and 1 mM MgCl2.

*c. Simultaneous polymerization and depolymerization of MTs.* After the respective incubation period, the MTP solution was divided into parts of 25 $\mu$l and each part was supplemented with, (1) a dilution of Kip3-eGFP ranging from $0-400$ nM, (2) 10 mM ATP (Roche), (3) 0.2 mg/ml casein (Sigma) and 0.1% Tween20 (Merck) for 1 hour at 27 °C. ATP enabled active motility of Kip3-eGFP to the MT plus ends and the casein as well as Tween20 prevented clustering and denaturing of the Kip3 motors. After 1 hour the Kip3-MT interaction in the 25 $\mu$l parts was terminated by addition of 300 mM KCl. After 1 minute incubation time, 1 $\mu$l of the solution was added to the imaging solution (BRB80 with 0.2 mg/ml DTT [Sigma], 40 mM glucose [Sigma], 110 mg/ml glucose oxidase [Serva] and 22 mg/ml catalase[Sigma]).

*d. Sample preparation for imaging MT length distribution.* To image the MTs, microfluidic flow channels were constructed, as described in Korten et al. [27], using dichlorodimethylsilane (DDS) coated 18 mm $\times$ 18 mm glass coverslips (Menzel, Braunschweig, Germany; #1.5) on DDS coated 22 mm $\times$ 22 mm coverslips separated by parafilm. Typically, each coverslip contained four flow channels with dimensions of 18 mm $\times$ 2 mm $\times$ 100 $\mu$m. The channels were flushed with a sequence of: (i) antibody solution consisting of 3 mg/ml anti-beta tubulin antibody (SAP.4G5, Sigma) in PBS in order to unspecifically bind antibodies to the surface (incubation time 5 minutes), (ii) Pluronic F127 (Sigma, 1% in PBS) in order to block the surface from unspecific protein adsorption (incubation time $>$ 60 minutes), (iii) 4 times BRB80 buffer to remove excess F127 in solution and exchange buffers, (iv) imaging solution, with 1 $\mu$l of the different 25 $\mu$l parts (MT polymerization mixture + varying concentrations of Kip3-eGFP) incubated for 2 minutes to allow MTs and free tubulin to attach to the surface, and (v) imaging solution to remove the MTs and free tubulin still in solution.

*e. Image acquisition.* Optical imaging was performed using an inverted fluorescence microscope (Zeiss, Axio Observer Z3, Carl Zeiss, Göttingen, Germany) with a 63x oil immersion 1.46 NA objective (Zeiss) in combination with an electron-multiplied charge-coupled device camera (Andor iXon Plus, Andor Technology, Belfast, UK) controlled by Metamorph (Molecular Devices Corporation, Sunnyvale, CA, USA). A Lumen 200 metal arc lamp (Prior Scientific Instruments Ltd., Cambridge, UK) was used for epifluorescence excitation. Rhodamine-labeled MTs immobilized on the surface were imaged using a TRITC filterset (Ex 534/30x, DC BC R561, EM BL593/40, all Chroma Technology Corp., Rockingham, VT) with an exposure time of 200 ms per frame. 20 images were acquired at different regions to scan the entire channel.

*f. Image Analysis.* Image analysis was performed using FIESTA tracking software [28] to track individual MTs in every imaged frame and obtain their length with nanometer precision. MTs smaller than 500 nm were ignored (visually not very different from potential tubulin clusters) from the image analysis leading to undersampling at lower microtubule lengths ($<$ 500 nm). Statistics performed on the MT lengths are discussed in the experimental results.

*g. Measurement of tubulin concentration incorporated in MTs.* To measure the concentration of free tubulin in the MTP solution after incubation times of 1.5 hours and 3 hours, the solutions were centrifuged using a Beckman airfuge (Beckman, Brea, CA) at 100,000g for 10 minutes. SDS-PAGE gel analysis was performed on the supernatant (free tubulin in MTP solution), the pellet (resuspended in 100 $\mu$l BRB80) and stock tubulin (diluted in 100 $\mu$l BRB80). The intensities of the gel bands were measured using ImageJ to obtain estimates of the percentages of tubulin incorporated in the polymerized MTs (see Fig. S16).

## S.VII. VARIABILITY IN EXPERIMENTAL DATA

*a. Number of MTs in per field of view.* This is a qualitative indicator of the density of MTs growing in the MTP solution under different conditions. The number of MTs attaching on the channel surface depends on the density of anti-beta tubulin antibodies adsorbed on the channel surface which in turn depends on (i) the hydrophobicity of the glass coverslips, (ii) the volume in the channel (built manually) and (ii) the time of incubation of antibodies in the channel. Variations in these factors could be minimized in a single experimental set allowing us to still infer the relative difference in MT density induced by different concentrations of Kip3. However, it is difficult to compare different sets of experiments.

*b. Initial MT length distribution in Control experiments.* MT growth is extremely sensitive to the time of polymerization, concentration of tubulin, temperature,

ionic strength and pH of the growth solution. While efforts were made to keep the conditions similar between different experimental sets, the initial MT length distribution before addition of Kip3 still varied significantly, as can be seen in Fig. S20.

*c. Microtubule length distribution.* While separating the MTP solution, mixing reagents (ATP, Kip3 solution, casein, Tween20, KCl, etc.), diluting the solution and flushing the solution into the channels, few MTs would break due to the shear forces generated. Therefore, it is possible that the number of short MTs is slightly overestimated in the length histograms.

*d. Amount of active Kip3 motors.* The Kip3 concentration indicated in the experiments is the amount of protein added to the solution and not the concentration of active Kip3 motors. Unfortunately, it is impossible to prevent the inactivation of a percentage of motors during the purification, snap-freezing and thawing process. Further, one would expect some motor clustering as well. The motor is soluble in a high ionic strength buffer but in the BRB80 solution used in the MTP solution, motors tend to cluster. To minimize the clustering of motors casein, Tween20 and a high concentration (10 mM) of ATP was added in the MTP solution. Due to the above reasons, it is not possible to quantitatively compare the theoretical and experimental values for Kip3 concentration.

## S.VIII. SUPPLEMENTARY FIGURES

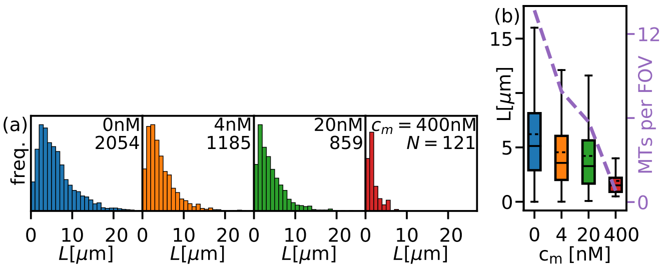


FIG. S15. Length distribution of MTs grown for 1.5 hours followed by addition of 0 nM, 4 nM, 20 nM and 400 nM Kip3 for 1 hour. (a) MTs have a median length of 5 $\mu$m (iqr=5 $\mu$m) when no Kip3 is added. Histograms of MT lengths (bin size = 1 $\mu$m) at different Kip3 concentrations indicate that MTs remain in the short length regime with the median MT length going down on increasing the Kip3 concentration, as seen in the box plots (b). As seen from the dashed line (right scale) of panel (b), the average number of MTs per imaged frame decreases with the concentration of Kip3.

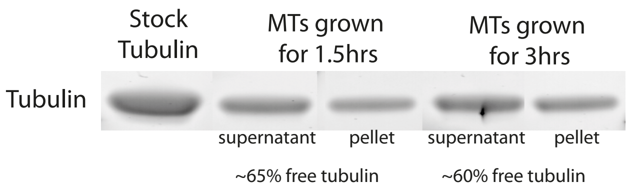


FIG. S16. Percentage of free tubulin in solution. MTs were grown for 1.5 hours and 3 hours and centrifuged to separate the free tubulin (supernatant) from the tubulin incorporated in MTs (pellet) and an SDS gel was performed. The intensities of the supernatant and the pellet indicate that MTs grown for 1.5 hours have ~65% free tubulin while MTs grown for 3 hours have ~60% free tubulin. The intensities of the supernatant and the pellet approximately add up to the intensity for the stock tubulin.

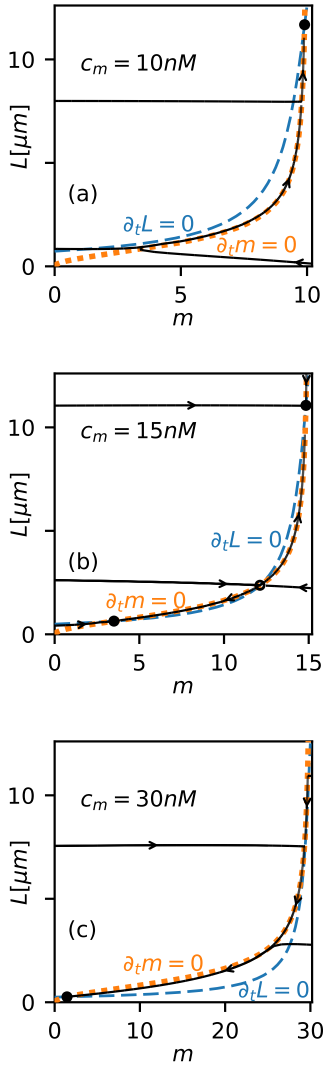


FIG. S17. Plots of representative stream lines of the vector field $(\partial_t m, \partial_t L)$ as from Eqs. (2) in the main text, for the three different motor concentrations of Fig. 3c in the main text at tubulin concentration $c_T = 1.5$ $\mu$M. Here, the approximate mean-field theory result for the flux off the MT, Eq. (4) in the main text, was used. The null clines $\partial_t m = 0$ and $\partial_t L = 0$ are also shown, cf. Fig. S3. For all three concentrations, the stream lines are almost horizontal until they approach the cline $\partial_t m = 0$. This implies that the dynamics of $m$ are much faster than those of $L$. This is due to the fact that motor binding and unbinding is possible at every binding site along the whole lattice, whereas MT elongation and shrinkage occur at the plus end only. Once the number of motors on the MT is quasi-stationary, the MT slowly adapts its length until its state reaches a fixed point. Because this effectively restricts the MT-motor dynamics to the nullcline $\partial_t m = 0$, a reduction to this subspace is possible, which was used in Fig. 3c in the main text. In parts (a) and (c), only a single fixed point exists, and a MT at these motor concentrations will always approach the uniquely defined stationary state. By contrast, for the intermediate motor concentration displayed in part (b), two fixed points at the north east, and south west of the diagram are present. In the middle, the separatrix and the corresponding saddle point divide phase space into regions attracted by the respective fixed points.

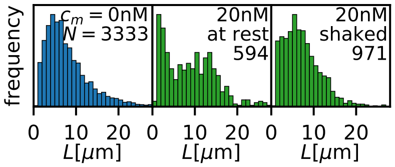


FIG. S18. Constant mixing of the MT-Kip3 solution changes the length distribution. 20 nM Kip3 were added to a solution of MTs which were pre-grown for 3 hours. One part of the resulting solution was left at rest for another hour, a second part was constantly mixed in a shaker for the same time. The resulting length distributions are strikingly different: While a bimodal distribution is observed for the part at rest, we find a unimodal distribution for the solution mixed in a shaker. This supports our interpretation of bistability: MTs jointly evolve to either the long or the short stationary length, as long as the system is so small that all resources are well-mixed. MTs at two different lengths can therefore only coexist in a solution when spatially separated domains exist in a large system. When a system is constantly mixed, we can assume that it behaves well-mixed on all length scales. As a consequence, only a single characteristic length is observed in the system.

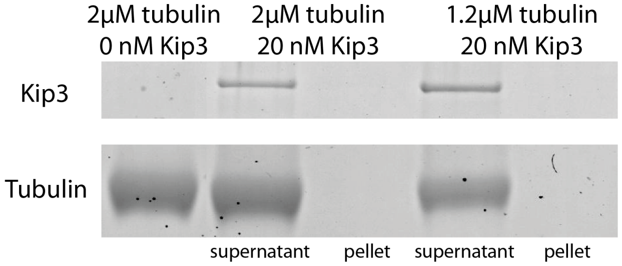


FIG. S19. MTs do not nucleate in the presence of Kip3. 20 nM Kip3 were added to solutions of 2 $\mu$M and 1.2 $\mu$M of tubulin. Here, the latter concentration approximately corresponds to the amount of free tubulin remaining in solution after MTs have formed in the absence of Kip3, cf. Fig. S16. Each solution was centrifuged after incubation of 1 hour, the supernatant and pellet were separated and an SDS gel was performed. We find that the intensity of the supernatant greatly exceeds the intensity of the pellet, both for Kip3 and tubulin. This indicates that (almost) all tubulin and Kip3 is free at these conditions. MTs therefore do not nucleate in the presence of 20 nM Kip3.

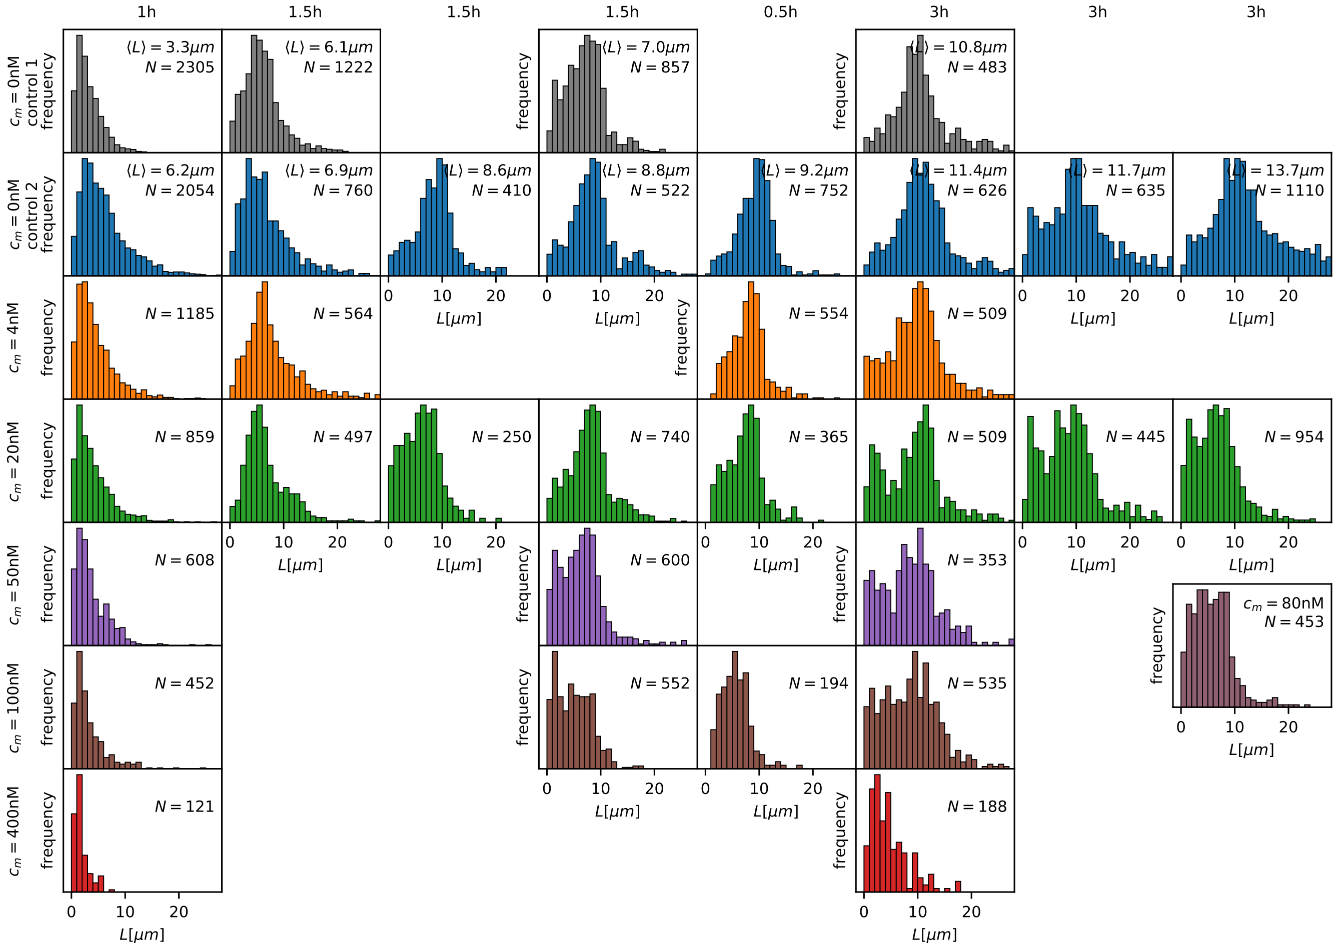


FIG. S20. Overview of the experimental measurements. Shown are MT length distributions recorded in various experiments at different conditions. For each column, the same initial solution was used, and varying amounts of Kip3 were added to a solution of MTs pre-grown for a specific amount of time (indicated in the column head). Varying the polymerization time of MTs in the absence impacts on the length distribution (control 1; MTs imaged directly at the time point when Kip3 is added to the other parts), although precise control of the average length is not possible in this way, see Sec. S.VIIb for details. Subsequent to initial growth, MTs were incubated without (control 2), or with Kip3 for another hour. The columns are ordered by the MTs' average length, when no Kip3 was added (control 2). We find that for short initial lengths, all length distributions are unimodal. In contrast, for longer initial MT lengths, distributions at certain motor concentrations become bimodal. The most prominent qualitatively difference is found for $c_m = 20$ nM and 50 nM.

[1] A. Parmeggiani, T. Franosch, and E. Frey, Phys. Rev. Lett. **90**, 086601 (2003).
[2] A. Parmeggiani, T. Franosch, and E. Frey, Phys. Rev. E **70**, 046101 (2004).
[3] Note that here, unlike in Ref. [2], $x$ runs from 0 to $L$.
[4] Here we leave out the Meissner phase found in Ref. [2] where the bulk behavior is independent of the rates at the boundaries, because we do not observe this phase at our conditions.
[5] J. Krug, Phys. Rev. Lett. **67**, 1882 (1991).
[6] A. B. Kolomeisky, G. M. Schütz, E. B. Kolomeisky, and J. P. Straley, J. Phys. A **31**, 6911 (1998).
[7] A. Melbinger, L. Reese, and E. Frey, Phys. Rev. Lett. **108**, 258104 (2012).
[8] E. Frey, A. Parmeggiani, and T. Franosch, Genome Inf. Ser. **15**, 46 (2004).
[9] S. H. Strogatz, *Nonlinear Dynamics and Chaos* (Westview Press, Boulder, CO, 2014).
[10] V. Varga, C. Leduc, V. Bormuth, S. Diez, and J. Howard, Cell **138**, 1174 (2009).
[11] A. A. Hyman, D. Chrétien, I. Arnal, and R. H. Wade, J. Cell Biol. **128**, 117 (1995).
[12] A. A. Hyman, S. Salser, D. N. Drechsel, N. Unwin, and T. J. Mitchison, Mol. Biol. Cell **3**, 1155 (1992).
[13] G. J. Brouhard, J. H. Stear, T. L. Noetzel, J. Al-Bassam, K. Kinoshita, S. C. Harrison, J. Howard, and A. A. Hyman, Cell **132**, 79 (2008).
[14] M. K. Gardner, B. D. Charlebois, I. M. Jánosi, J. Howard, A. J. Hunt, and D. J. Odde, Cell **146**, 582 (2011).
[15] I. A. Telley, P. Bieling, and T. Surrey, Biophys. J. **96**, 3341 (2009).
[16] R. Schneider, T. Korten, W. J. Walter, and S. Diez, Biophys. J. **108**, 2249 (2015).
[17] The large deviation of these numbers reflects that the length distributions of pre-grown MTs can be very different, even if they are grown for the same time.
[18] I. R. Graf and E. Frey, Phys. Rev. Lett. **118**, 128101 (2017).
[19] J. Halatek and E. Frey, Cell Rep. **1**, 741 (2012).
[20] J. Halatek and E. Frey, Nat. Phys. (2018), DOI: 10.1038/s41567-017-0040-5.
[21] E. D. Salmon, W. M. Saxton, R. J. Leslie, M. L. Karow, and J. R. McIntosh, J. Cell Biol. **99**, 2157 (1984).
[22] J. Hazel, K. Krutkramelis, P. Mooney, M. Tomschik, K. Gerow, J. Oakey, and J. C. Gatlin, Science **342**, 853 (2013).
[23] M. C. Good, M. D. Vahey, A. Skandarajah, D. A. Fletcher, and R. Heald, Science **342**, 856 (2013), arXiv:20.
[24] C. Leduc, K. Padberg-Gehle, V. Varga, D. Helbing, S. Diez, and J. Howard, Proc. Natl. Acad. Sci. U.S.A. **109**, 6100 (2012).
[25] M. Castoldi and A. V. Popov, Protein Expression Purif. **32**, 83 (2003).
[26] V. Varga, J. Helenius, K. Tanaka, A. A. Hyman, T. U. Tanaka, and J. Howard, Nat. Cell Biol. **8**, 957 (2006).
[27] T. Korten, B. Nitzsche, C. Gell, F. Ruhnow, C. Leduc, and S. Diez, in *Single Molecule Analysis: Methods and Protocols*, edited by E. J. G. Peterman and G. J. L. Wuite (Humana Press, Totowa, NJ, 2011) p. 121.
[28] F. Ruhnow, D. Zwicker, and S. Diez, Biophys. J. **100**, 2820 (2011).
